# Supplementary material for: Enabling Weak Client Participation via On-device Knowledge Distillation in Heterogeneous Federated Learning
Source: arXiv:2503.11151 source file (2026-01-08)
Supplement: Supplementary file 1 [file appendix.tex]

\section{Appendix}
\subsection {Additional Experimental Results}
We use TensorFlow 2.13.0 and MPI (OpenMPI 4.1.5) for FL simulation.
All experiments run on a GPU cluster that contains 2 NVIDIA A6000 GPUs.
For all the methods in our comparative study, the algorithm-specific hyper-parameters were highly tuned using appropriate grid searches (See Appendix for the details).
For CIFAR-100 fine-tuning, we freeze the transformer pre-trained on ImageNet and train the output-side two fully-connected layers only.

\subsection{Data Preprocessing}
Some benchmark datasets require a couple of preprocessing steps so that the model can effectively learn meaningful knowledge.
\\
\textbf{CIFAR-10, CIFAR-100} -- We perform the typical image preprocessing used in many previous works.
First, each image is padded by 4 pixels on every dimension and then randomly cropped to the original size.
Then, we normalize and standardize the values for all individual pixels.
Finally, we randomly flip the image horizontally with a probability of 0.5.
\\
\textbf{Google Speech Command} -- We apply a few audio preprocessing steps to each \textit{wav} file.
First, the raw data is decoded and read into the memory space.
Second, we zero out all the values that lie below 18,000 samples (1 sec).
Finally, we apply short-time fourier transform to the data to get a spectrogram.
In this way, each \textit{wav} file is converted into a 2-D spectrogram matrix, which can be directly fed into the model for training.

\subsection{Algorithm-Specific Hyper-Parameter Settings}
To improve the reproducibility, we provide the detailed hyper-parameter settings we used when measuring the SOTA algorithms' FL performance.
We summarize the hyper-parameter settings corresponding to Table~\ref{tab:base} in \Cref{tab:cifar10,tab:femnist,tab:cifar100,tab:imdb,tab:gspeech}.
The hyper-parameter settings corresponding to Table~\ref{tab:compare} are shown in \Cref{tab:sotacifar10,tab:sotafemnist,tab:sotagspeech}.
\\
\textbf{Homogeneous FL methods} -- For the algorithms that do not run KD (FedAvg and MOON), the number of local steps is set to $2\tau$ while all the others run $\tau$ SGD steps and then $\tau$ KD steps.
Although it does not guarantee exactly the same computational cost across the algorithms, it allows them to have at least a similar workload.
MOON is an advanced FL optimization algorithm that redesigns the loss function to address the data heterogeneity issue.
%However, it is designed only for computer vision tasks and not applicable to other NLP and audio recognition tasks.
However, it is designed only for computer vision tasks, and thus we evaluate its performance and compare to our method in computer vision benchmarks only.
%MOON is originally designed for computer vision tasks, but we apply this to all the benchmarks including audio classification (Google Speech).
\\
\textbf{FedMD} -- When running FedMD, we found that the transfer learning with private data achieves better accuracy when the learning rate is much smaller than the training with public data.
Thus, we do not re-initialize the learning rate after the learning rate decay in the transfer learning with public data and just use the small learning rate during the transfer learning with private data.
\\
\textbf{FedGEM} -- FedGEM has a weight factor $\epsilon$ which determines how much KL contributes to the total loss.
We set $\epsilon$ to 0.75 as the original authors presented in \cite{cheng2021fedgems}.
FedGEM also uses a relatively smaller number of local steps $\tau$ compared to other SOTA algorithms. 
Because FedGEM has three training rounds in total, two at the edge and one at the server-side, we set the $\tau$ to make the total steps the same as other algorithms.
For example, in FEMNIST experiments, FedAvg runs 60 steps, FedDF runs 30 SGD steps + 30 KD steps, and FedGEM runs 20 + 20 client steps and 20 server steps.
While conducting experiments with FedGEM and DS-FL on the CIFAR-10, we observed that decaying the learning rate does not result in any significant changes in accuracy.
Therefore, we use a fixed learning rate without decay.
\\
\textbf{Proposed Method} -- We found that a small KL coefficient $\lambda$ helps improve our method accuracy.
Instead of using a constant setting, we employed a structured coefficient control method proposed in~\cite{wu2021peer}.
We applied this to other SOTA methods, however, we have not observed any meaningful accuracy improvements.

\subsection {Ablation Study Settings}
In an ablation study with a varying number of strong clients, the public data should be partitioned up to 40 subsets (we consider the cases where the number of clients is 10, 20, or 40).
Due to the large number of clients, if the Dirichlet concentration coefficient is 0.1, it gives 0 samples to some clients.
Thus, we use $\alpha = 0.2$ instead in this experiment only.

\begin{table}[h]
\footnotesize
\centering
\caption{
    CIFAR-10 Hyper-Parameter Settings
}
\label{tab:cifar10}
\begin{tabular}{lccc} \toprule
Hyperparameters & Weak-only & Strong - only  & Proposed \\ \midrule
{model size}& {25\%} & {100\%} & {100\%}\\
{$\tau$ (local steps)}& \multicolumn{3}{c}{60} \\
{batch size}& \multicolumn{3}{c}{32} \\ % Merging 3 columns
{learning rate}& \multicolumn{3}{c}{0.2, 0.02(200 epoch), 0.002(300 epoch)} \\ % Merging 3 columns
{total epoch}& \multicolumn{3}{c}{400} \\ % Merging 3 columns
{weight decay}& \multicolumn{3}{c}{0.0001} \\ % Merging 3 columns
{temperature}& \multicolumn{3}{c}{3} \\ % Merging 3 columns
{epoch threshold for $\lambda$ ramp-up}& \multicolumn{3}{c}{300} \\ % Merging 3 columns
{$\lambda$ (KL coefficient)}& \multicolumn{3}{c}{0.5} \\ % Merging 3 columns
{$\alpha$ (Dirichlet coefficient)}& \multicolumn{3}{c}{0.1} \\ % Merging 3 columns
\bottomrule
\end{tabular}
\end{table}

\begin{table}[th]
\footnotesize
\centering
\caption{
    FEMNIST Hyper-Parameter Settings
}
\label{tab:femnist}
\begin{tabular}{lccc} \toprule
Hyperparameters & Weak-only & Strong - only  & Proposed \\ \midrule
{model size}& {25\%} & {100\%} & {100\%}\\
{$\tau$ (local steps)}& \multicolumn{3}{c}{60}\\
{batch size}& \multicolumn{3}{c}{20} \\ % Merging 3 columns
{learning rate}& \multicolumn{3}{c}{0.02} \\ % Merging 3 columns
{total epoch}& \multicolumn{3}{c}{200} \\ % Merging 3 columns
{weight decay}& \multicolumn{3}{c}{0.0001} \\ % Merging 3 columns
{temperature}& \multicolumn{3}{c}{3} \\ % Merging 3 columns
{$\lambda$ (KL coefficient)}& \multicolumn{3}{c}{1} \\ % Merging 3 columns
{$\alpha$ (Dirichlet coefficient)}& \multicolumn{3}{c}{0.1} \\ % Merging 3 columns
\bottomrule
\end{tabular}
\end{table}

\begin{table}[th]
\footnotesize
\centering
\caption{
    CIFAR-100 (Fine-tuning) Hyper-Parameters
}
\label{tab:cifar100}
\begin{tabular}{lccc} \toprule
Hyperparameters & Weak-only & Strong - only  & Proposed \\ \midrule
{model}& {ResNet50} & {ViT-b16} & {ViT-b16}\\
{$\tau$ (local steps)}& \multicolumn{3}{c}{120}\\
{batch size}& \multicolumn{3}{c}{32} \\ % Merging 3 columns
{learning rate}& \multicolumn{3}{c}{0.04, 0.004(25 epoch), 0.0004(35 epoch)} \\ % Merging 3 columns
{total epoch}& \multicolumn{3}{c}{40} \\ % Merging 3 columns
{weight decay}& \multicolumn{3}{c}{0.0005} \\ % Merging 3 columns
{temperature}& \multicolumn{3}{c}{1} \\ % Merging 3 columns
{$\lambda$ (KL coefficient)}& \multicolumn{3}{c}{1} \\ % Merging 3 columns
{$\alpha$ (Dirichlet coefficient)}& \multicolumn{3}{c}{0.1} \\ % Merging 3 columns
\bottomrule
\end{tabular}
\end{table}

\begin{table*}[th]
\footnotesize
\centering
\caption{
    IMDB review Hyper-Parameter Settings
}
\label{tab:imdb}
\begin{tabular}{lccc} \toprule
Hyperparameters & Weak-only & Strong - only  & Proposed \\ \midrule
{model size}& {25\%} & {100\%} & {100\%}\\
{$\tau$ (local steps)}& \multicolumn{3}{c}{40} \\
{batch size}& \multicolumn{3}{c}{10} \\ % Merging 3 columns
{learning rate}& \multicolumn{3}{c}{0.4} \\ % Merging 3 columns
{total epoch}& \multicolumn{3}{c}{90} \\ % Merging 3 columns
{weight decay}& \multicolumn{3}{c}{0.0001} \\ % Merging 3 columns
{temperature}& \multicolumn{3}{c}{1} \\ % Merging 3 columns
{epoch threshold for $\lambda$ ramp-up }& \multicolumn{3}{c}{80} \\ % Merging 3 columns
{$\lambda$ (KL coefficient)}& \multicolumn{3}{c}{1} \\ % Merging 3 columns
{$\alpha$ (Dirichlet coefficient)}& \multicolumn{3}{c}{0.1} \\ % Merging 3 columns
\bottomrule
\end{tabular}
\end{table*}

\begin{table*}[th]
\footnotesize
\centering
\caption{
    Google Speech Hyper-Parameter Settings
}
\label{tab:gspeech}
\begin{tabular}{lccc} \toprule
Hyperparameters & Weak-only & Strong - only  & Proposed \\ \midrule
{model size}& {25\%} & {100\%} & {100\%}\\
{$\tau$ (local steps)}& \multicolumn{3}{c}{80}\\
{batch size}& \multicolumn{3}{c}{32} \\ % Merging 3 columns
{learning rate}& \multicolumn{3}{c}{0.02, 0.002 (80 epoch)} \\ % Merging 3 columns
{total epoch}& \multicolumn{3}{c}{100} \\ % Merging 3 columns
{weight decay}& \multicolumn{3}{c}{0.0001} \\ % Merging 3 columns
{temperature}& \multicolumn{3}{c}{1} \\ % Merging 3 columns
{epoch threshold for $\lambda$ ramp-up}& \multicolumn{3}{c}{80} \\ % Merging 3 columns
{$\lambda$ (KL coefficient)}& \multicolumn{3}{c}{1} \\ % Merging 3 columns
{$\alpha$ (Dirichlet coefficient)}& \multicolumn{3}{c}{0.1} \\ % Merging 3 columns
\bottomrule
\end{tabular}
\end{table*}

\begin{table*}[t]
\footnotesize
\centering
\caption{
    CIFAR-10 Hyper-Parameter Settings for SOTA FL Methods
}
\label{tab:sotacifar10}
\begin{tabular}{lccccccc} \toprule
Hyperparameters & FedAvg & MOON & FedDF & DS-FL & FedMD & FedGEM & Proposed \\ \midrule
\multirow{2}{*}{client model size}& \multirow{2}{*}{25\%} &\multirow{2}{*} {25\%} &\multirow{2}{*} {25\%}& {80 clients: 25\%}& {80 clients: 25\%}& {80 clients: 25\%}& {80 clients: 25\%}\\
&&&&{20 clients: 100\%}& {20 clients: 100\%}& {20 clients: 100\%}& {20 clients: 100\%}\\
{server model size}& {25\%} & {25\%}  & {25\%}& {N/A}&{N/A}&{100\%}&{N/A}\\
{$\tau$ (local steps)}&{90} & {90} & {90}& {90}& {90} & {90}& {90}\\
{learning rate}& {0.2} &{0.2} &{0.2} &{0.01}&{0.2}&{0.05}&{0.2}\\ % Merging 3 columns
{temperature}&{N/A}&{N/A}&{1} & {1} &{1} & {1}&{3}\\ % Merging 3 columns
{batch size}& \multicolumn{7}{c}{32} \\ % Merging 3 columns
{total epoch}& \multicolumn{7}{c}{400} \\ % Merging 3 columns
{weight decay}& \multicolumn{7}{c}{0.0001} \\ % Merging 3 columns
\bottomrule
\end{tabular}
\end{table*}

\begin{table*}[t]
\footnotesize
\centering
\caption{
    FEMNIST Hyper-Parameter Settings for SOTA FL Methods
}
\label{tab:sotafemnist}
\begin{tabular}{lccccccc} \toprule
Hyperparameters & FedAvg & MOON & FedDF & DS-FL & FedMD & FedGEM & Proposed \\ \midrule
\multirow{2}{*}{client model size}& \multirow{2}{*}{25\%} &\multirow{2}{*} {25\%} &\multirow{2}{*} {25\%}& {80 clients: 25\%}& {80 clients: 25\%}& {80 clients: 25\%}& {80 clients: 25\%}\\
&&&&{20 clients: 100\%}& {20 clients: 100\%}& {20 clients: 100\%}& {20 clients: 100\%}\\
{server model size}& {25\%} & {25\%}  & {25\%}& {N/A}&{N/A}&{100\%}&{N/A}\\
{$\tau$ (local steps)}&{90} & {90} & {90}& {90}& {90} & {90}& {90}\\
{learning rate}& {0.02}& {0.02}& {0.01} &{0.01}&{0.01}&{0.01}&{0.02}\\ % Merging 3 columns
{temperature}&{N/A}&{N/A}&{1} & {1} &{1} & {1}&{3}\\ % Merging 3 columns 
{batch size}& \multicolumn{7}{c}{20} \\ % Merging 3 columns
{total epoch}& \multicolumn{7}{c}{200} \\ % Merging 3 columns
{weight decay}& \multicolumn{7}{c}{0.0001} \\ % Merging 3 columns
\bottomrule
\end{tabular}
\end{table*}

\begin{table*}[t]
\footnotesize
\centering
\caption{
    Google Speech Hyper-Parameter Settings for SOTA FL Methods
}
\label{tab:sotagspeech}
\begin{tabular}{lccccccc} \toprule
Hyperparameters & FedAvg & MOON & FedDF & DS-FL & FedMD & FedGEM & Proposed \\ \midrule
\multirow{2}{*}{client model size}& \multirow{2}{*}{25\%} & N/A &\multirow{2}{*} {25\%}& {80 clients: 25\%}& {80 clients: 25\%}& {80 clients: 25\%}& {80 clients: 25\%}\\
&&&&{20 clients: 100\%}& {20 clients: 100\%}& {20 clients: 100\%}& {20 clients: 100\%}\\
{server model size}& {25\%} & N/A  & {25\%}& {N/A}&{N/A}&{100\%}&{N/A}\\
{$\tau$ (local steps)}& {120} & N/A & {120}& {120}& {120} & {120} & {120}\\
{learning rate}& 0.02 & N/A & 0.02 & 0.01 & 0.02 & 0.02 & 0.02  \\ % Merging 3 columns
{temperature}& \multicolumn{7}{c}{1}\\ % Merging 3 columns
{batch size}& \multicolumn{7}{c}{32} \\ % Merging 3 columns
{total epoch}& \multicolumn{7}{c}{100} \\ % Merging 3 columns
{weight decay}& \multicolumn{7}{c}{0.0001} \\ % Merging 3 columns
\bottomrule
\end{tabular}
\end{table*}
